# Supplementary material for: Efficient Event-Based Object Detection: A Hybrid Neural Network with Spatial and Temporal Attention
Source: arXiv:2403.10173 source file (2025-06-19)
Supplement: Supplementary file 1 [file supple.pdf]

# Supplementary Materials for A Hybrid SNN-ANN Network for Event-based Object Detection with Spatial and Temporal Attention

Soikat Hasan Ahmed<sup>1,2</sup>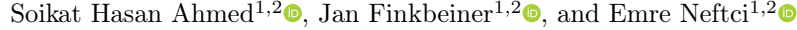, Jan Finkbeiner<sup>1,2</sup>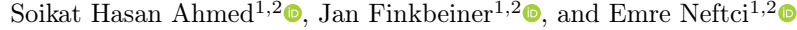, and Emre Neftci<sup>1,2</sup>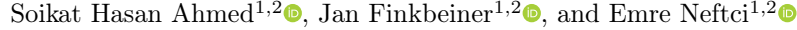

<sup>1</sup> Forschungszentrum Jülich

<sup>2</sup> RWTH Aachen, Germany

{s.ahmed,j.finkbeiner,e.neftci}@fz-juelich.de

**Abstract.** Event cameras offer high temporal resolution and dynamic range with minimal motion blur, making them promising for object detection tasks. While Spiking Neural Networks (SNNs) are a natural match for event-based sensory data and enable ultra-energy efficient and low latency inference on neuromorphic hardware, Artificial Neural Networks (ANNs) tend to display more stable training dynamics and faster convergence resulting in greater task performance. Hybrid SNN-ANN approaches are a promising alternative, enabling to leverage the strengths of both SNN and ANN architectures. In this work, we introduce the first Hybrid Attention-based SNN-ANN backbone for object detection using event cameras. We propose a novel Attention-based SNN-ANN bridge module to capture sparse spatial and temporal relations from the SNN layer and convert them into dense feature maps for the ANN part of the backbone. Experimental results demonstrate that our proposed method surpasses baseline hybrid and SNN-based approaches by significant margins, with results comparable to existing ANN-based methods. Extensive ablation studies confirm the effectiveness of our proposed modules and architectural choices. These results pave the way toward a hybrid SNN-ANN architecture that achieves ANN-like performance at a drastically reduced parameter budget. We implemented the SNN blocks on digital neuromorphic hardware to investigate latency and power consumption and demonstrate the feasibility of our approach.

## 1 Supplementary Details

The supplementary material accompanies the manuscript titled "A Hybrid SNN-ANN Network for Event-based Object Detection with Spatial and Temporal Attention" and includes the architecture details of the proposed hybrid backbone network as well as hardware performance details.

### 1.1 Network Architecture

Tab. 1 displays the network architecture of the proposed hybrid backbone. Additionally, Fig. 1 illustrates the basic SNN and ANN blocks. For better understand-

ing, we have also included an additional figure (Fig. 2) to clarify the channel-wise temporal grouping operation from Spatial-aware Temporal attention, where similar features from different time dimensions are grouped.

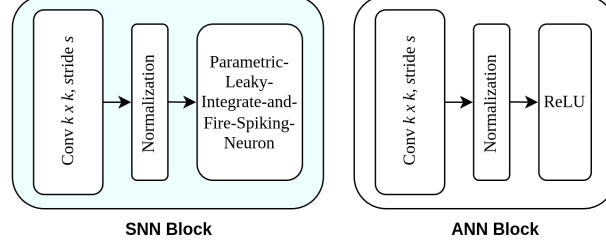

**Fig. 1:** Basic SNN and ANN blocks.

**Table 1:** Hybrid backbone architecture, where the kernel  $XcKpZsS$  represents  $X$  convolution filters of size  $K \times K$  with padding  $Z$  and stride  $S$ .

| Layer                    | Kernel    | Output Dimensions                                      | Layer Type   |
|--------------------------|-----------|--------------------------------------------------------|--------------|
| Input                    | -         | $T \times 2 \times H \times W$                         |              |
| 1                        | 64c3p1s2  | $T \times 64 \times \frac{1}{2}H \times \frac{1}{2}W$  | SNN Layers   |
| 2                        | 128c3p1s2 | $T \times 128 \times \frac{1}{4}H \times \frac{1}{4}W$ |              |
| 3                        | 256c3p1s2 | $T \times 256 \times \frac{1}{8}H \times \frac{1}{8}W$ |              |
| 4                        | 256c3p1s1 | $T \times 256 \times \frac{1}{8}H \times \frac{1}{8}W$ |              |
| 5                        | -         | $256 \times \frac{1}{8}H \times \frac{1}{8}W$          | <i>basab</i> |
| 6                        | 256c3p1s1 | $256 \times \frac{1}{8}H \times \frac{1}{8}W$          | ANN Layers   |
| 7                        | 256c3p1s2 | $256 \times \frac{1}{16}H \times \frac{1}{16}W$        |              |
| 8                        | 256c3p1s1 | $256 \times \frac{1}{16}H \times \frac{1}{16}W$        |              |
| 9                        | 256c3p1s2 | $256 \times \frac{1}{32}H \times \frac{1}{32}W$        |              |
| Detection Head YoloX [2] |           |                                                        |              |

## 1.2 Hardware Implementation

This section provides more performance details on the hardware implementation of the spiking layers of the backbone on a digital neuromorphic chip, Intel’s Loihi 2 [1]. In Tab. 3, we present the Power and time measurements of the SNN block on Loihi 2 for various input sizes, each tested with different weight quantization settings.

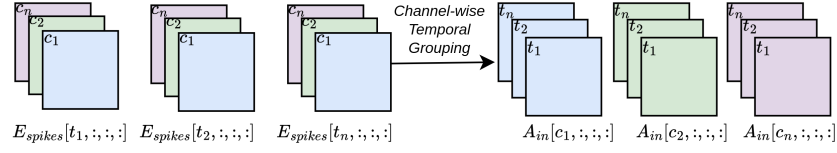

**Fig. 2:** Visualization of channel-wise temporal grouping.

**Table 2:** This table shows the effects of accuracy due to the quantization of the weights for the SNN blocks, aimed at making them compatible with neuromorphic hardware.

| Models              | mAP(.5) | mAP(.5:.05:.95) |
|---------------------|---------|-----------------|
| Variant 1 (float16) | 0.613   | 0.348           |
| Variant 2 (int8)    | 0.612   | 0.349           |
| Variant 3 (int6)    | 0.612   | 0.348           |
| Variant 4 (int4)    | 0.610   | 0.347           |
| Variant 5 (int2)    | 0.432   | 0.224           |

## References

1. Davies, M., Srinivasa, N., Lin, T.H., Chinya, G., Cao, Y., Choday, S.H., Dimou, G., Joshi, P., Imam, N., Jain, S., et al.: Loihi: A neuromorphic manycore processor with on-chip learning. *Ieee Micro* **38**(1), 82–99 (2018)
2. Ge, Z., Liu, S., Wang, F., Li, Z., Sun, J.: Yolox: Exceeding yolo series in 2021. *arXiv preprint arXiv:2107.08430* (2021)

**Table 3:** Power and time measurements of the SNN block on Loihi 2 for several input sizes and number of weight bits. The power is measured in Watts and the execution time per step in milliseconds. The mean and standard deviation of the measurements averaged over 12 inputs for a total of 100k steps are reported.

| Input size<br>(C,W,H) | Weight<br>qunatization | Number<br>of chips | Total Power [W] | Execution Time<br>Per Step [ms] |
|-----------------------|------------------------|--------------------|-----------------|---------------------------------|
| (2, 256, 160)         | int8                   | 6                  | $1.73 \pm 0.10$ | $2.06 \pm 0.74$                 |
|                       | int6                   | 6                  | $1.71 \pm 0.11$ | $2.06 \pm 0.74$                 |
|                       | int4                   | 6                  | $1.95 \pm 0.33$ | $1.16 \pm 0.49$                 |
| (2, 128, 160)         | int8                   | 4                  | $1.51 \pm 0.56$ | $0.80 \pm 0.32$                 |
|                       | int6                   | 4                  | $1.81 \pm 0.48$ | $0.45 \pm 0.18$                 |
|                       | int4                   | 3                  | $1.39 \pm 0.44$ | $0.49 \pm 0.18$                 |
